# Supplementary material for: StEP: Style-based Encoder Pre-training for Multi-modal Image Synthesis
Source: arXiv:2104.07098 source file (2021-04-14)
Supplement: Supplementary file 1 [file supplementary.tex]

\section{Supplementary material}
\label{sec:supp_material}

\subsection{User study}

We reported the results of a user study in the main text. The user study has five sections, each of which contains 50 questions comparing a pair of images from two methods.
We attach all images used in our study to the supplementary material zip file. Specifically, the zip file includes five folders corresponding to the five sections in our study.
The names of the folders indicate the two methods compared in them for short.
% Due to the limit of file size they have been compressed to JPEG format but the original ones in the questionnaire are all PNGs.
The order of two images in a question (left vs right) is randomly set. We are including a README file to specify the order for all questions.
Figure~\ref{fig:user_study} shows two example questions that are shown to the user as part of the instructions.
% We also set an example section at the beginning of the survey to clarify its purpose and content. The two example questions are shown in Figure~\ref{fig:user_study}.

\begin{figure*}[ht!]
    \centering
    \captionsetup[subfigure]{aboveskip=1pt,belowskip=3pt}
    \begin{subfigure}[b]{0.6\linewidth}
        \centering
        \includegraphics[width=\linewidth]{figures/user_study/user_study2.pdf}\\
        % \caption{Example question 1: which looks the more realistic, which is the main factor}
        \caption{Example question 1: realism is the main factor for choosing a preference.}
    \end{subfigure}
    \begin{subfigure}[b]{0.6\linewidth}
        \centering
        \includegraphics[width=\linewidth]{figures/user_study/user_study.pdf}\\
        \caption{Example question 2: if both outputs have the same level of realism, then the user chooses the output that better matches the style image.}
    \end{subfigure}

    % \caption{Each question shows a sketch of a shoe and below it a real shoe from which we want to capture the style (color and texture) and transfer it to the sketch. Bottom left and bottom right are the outputs of two different methods. Choose which method (Left vs Right) generates a more \textbf{realistic} output with similar style to that of the style image (middle). You should compare the two methods based on (a) which looks the more realistic, which is the main factor, and (b) if both have the same level of realism, then which one better matches the style image.}
    \caption{Instructions and sample questions given in our user study. Each question shows a sketch of a shoe and below it a real shoe from which we want to capture the style (color and texture) and transfer it to the sketch. Bottom left and bottom right are the outputs of two different methods. The user chooses which method (left vs right) generates a more realistic output with similar style to that of the style image (middle). The user compares the two methods based on (a) which looks the more realistic, and (b) if both have the same level of realism, then which one better matches the style image.}
    \label{fig:user_study}
\end{figure*}
% ========================================================================================================================
